# Supplementary material for: Robust optimal density control of robotic swarms
Source: arXiv:2205.12592 source file (2022-12-04)
Supplement: Supplementary file 1 [file appendix.tex]

\crl{The appendix can be cut out completely}

We test the reduced gradient computation of Algorithm  against centered finite differences, the numerical results are shown in Figure \ref{red_grad_check}.

\begin{figure}[h!]
\raggedright
\subfigure{\includegraphics[width=0.2\textwidth]{sim_results/grad_error.png}}
\subfigure{\includegraphics[width=0.2\textwidth]{sim_results/grad_comparison.png}}
\caption{Numerical comparison between central finite difference (very slow) and adjoint gradient computation of algorithm above. }
\label{red_grad_check}
\end{figure}

We now test the algorithm with an inverse problem to check the algorithm convergence to the global optimum. We select a control vector field $\hat{\mathbf{u}} = [x_1 \,\, x_2]^{\top}$ and compute the corresponding solution $\hat{q}$ and we set $z = \hat{q}$. Then we use Algorithm \crl{QN} to solve the resulting optimization problem. If $\beta$ is small enough the solution of the iterative algorithm $\mathbf{u}^{\star}$ converges to $\hat{\mathbf{u}}$ sufficiently far from the boundaries. Note that due to the structure of the optimal controls discussed in the previous section the optimal control is forced to be tangent to the domain and thus cannot converge to $\hat{\mathbf{u}}$ close to the boundary.

\begin{figure}[h!]
\raggedright
\subfigure{\includegraphics[width=0.2\textwidth]{sim_results/u_field_controlled.png}}
\subfigure{\includegraphics[width=0.2\textwidth]{sim_4/delta_u_field.png}}
\subfigure{\includegraphics[width=0.2\textwidth]{sim_4/Cost_conv.png}}
\subfigure{
\includegraphics[width=0.2\textwidth]{sim_4/Grad_conv.png}
}
\caption{add caption add caption}
\label{convergence_fom}
\end{figure}
